# Supplementary material for: MASH-VLM: Mitigating Action-Scene Hallucination in Video-LLMs through Disentangled Spatial-Temporal Representations
Source: arXiv:2503.15871 source file (2025-03-20)
Supplement: Supplementary file 1 [file suppl.tex]

% \documentclass[10pt,twocolumn,letterpaper]{article}
% \input{setup/package}
% \input{setup/macros}
% \input{setup/symbols}
% \input{setup/graphicspath}
% % \usepackage[review]{cvpr}  
% % % \usepackage{cvpr}


% %%%%%%%%% PAPER TYPE  - PLEASE UPDATE FOR FINAL VERSION
% % \usepackage[review]{cvpr}
% \usepackage{cvpr}

% \input{preamble}

% % \iccvfinalcopy % *** Uncomment this line for the final submission
% % Pages are numbered in submission mode, and unnumbered in camera-ready
% % \ifcvprfinal\pagestyle{empty}\fi
% \definecolor{cvprblue}{rgb}{0.21,0.49,0.74}
% \usepackage[pagebackref,breaklinks,colorlinks,allcolors=cvprblue]{hyperref}


% %%%%%%%%% PAPER ID  - PLEASE UPDATE
% %%%%%%%%% PAPER ID  - PLEASE UPDATE
% \def\paperID{14904} % *** Enter the Paper ID here
% \def\confName{CVPR}
% \def\confYear{2025}


% \def\httilde{\mbox{\tt\raisebox{-.5ex}{\symbol{126}}}}
% % \def\confName{ICCV}
% % \def\confYear{2023}


% % Pages are numbered in submission mode, and unnumbered in camera-ready
% % \ifcvprfinal\pagestyle{empty}\fi

% % ==============================================================
% % Main Document
% % ==============================================================

% \begin{document}

% \title{MASH-VLM: Mitigating Action-Scene Hallucination in Video-LLMs\\
% through Disentangled Spatial-Temporal Representations \\
% Supplementary Material}

% \maketitle
% \thispagestyle{empty}
% % Main paper

% \input{99_supp_content}
% % \clearpage
% % {
% % \small
% % \bibliographystyle{ieee_fullname}
% % \bibliography{main}
% % }
% \clearpage
% {
% \twocolumn[
% % \section*{References}
% ]
% \bibliographystyle{ieee_fullname}
% \bibliography{main}
% }

% \end{document}
